# Supplementary material for: MotionBridge: Dynamic Video Inbetweening with Flexible Controls
Source: arXiv:2412.13190 source file (2025-01-07)
Supplement: Supplementary file 1 [file main_results_supp.tex]

\begin{figure*}[t]
\centering
  \includegraphics[width=1\textwidth,height=\textheight]{data/results_main_small.pdf}
  \caption{Results of interpolation with motion vectors .}
  \label{fig:main_res_supp}
\end{figure*}
