# Supplementary material for: MotionBridge: Dynamic Video Inbetweening with Flexible Controls
Source: arXiv:2412.13190 source file (2025-01-07)
Supplement: Supplementary file 2 [file X_suppl.tex]

%new views of same object, i can use manual control here 

\subsection{}{Effect of more frames}

\todoc{move below three into supp, and add a new one for "Synthetic Video Refinement"}

\begin{figure}[t]
\centering
  \includegraphics[width=1\linewidth]{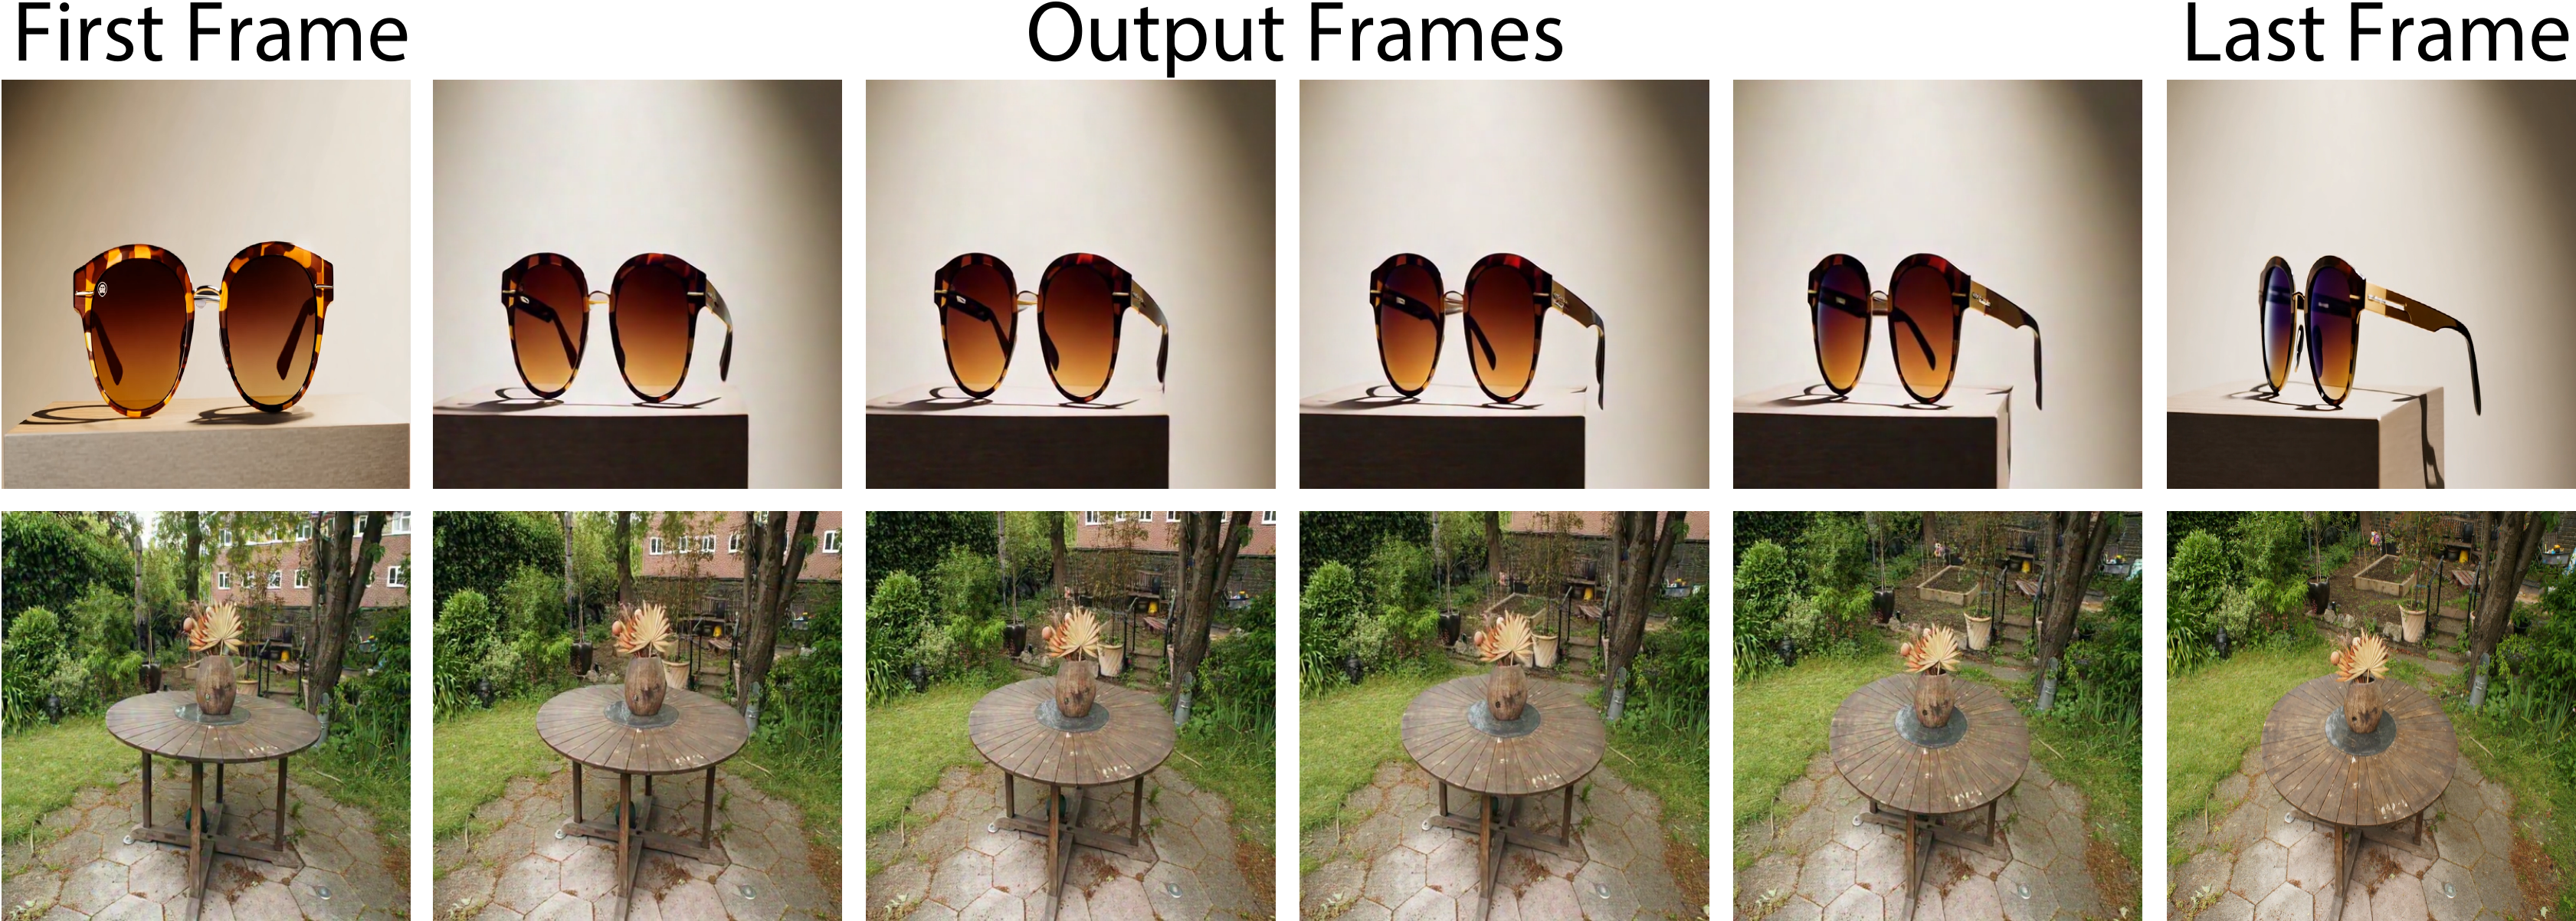}
  \caption{ 
  \mt{Camera motion results showing a smooth panning to interpolate the two frames.}
  }
  \label{fig:camera}
\end{figure}
\subsection{Camera Motion Generation}
\mt{Given two input frames of the same object from different camera locations, we use automatic motion extraction via optical flow to generate the inbetween frames in Fig.~\ref{fig:camera}}.

\begin{figure}[t]
\centering
  \includegraphics[width=1\linewidth]{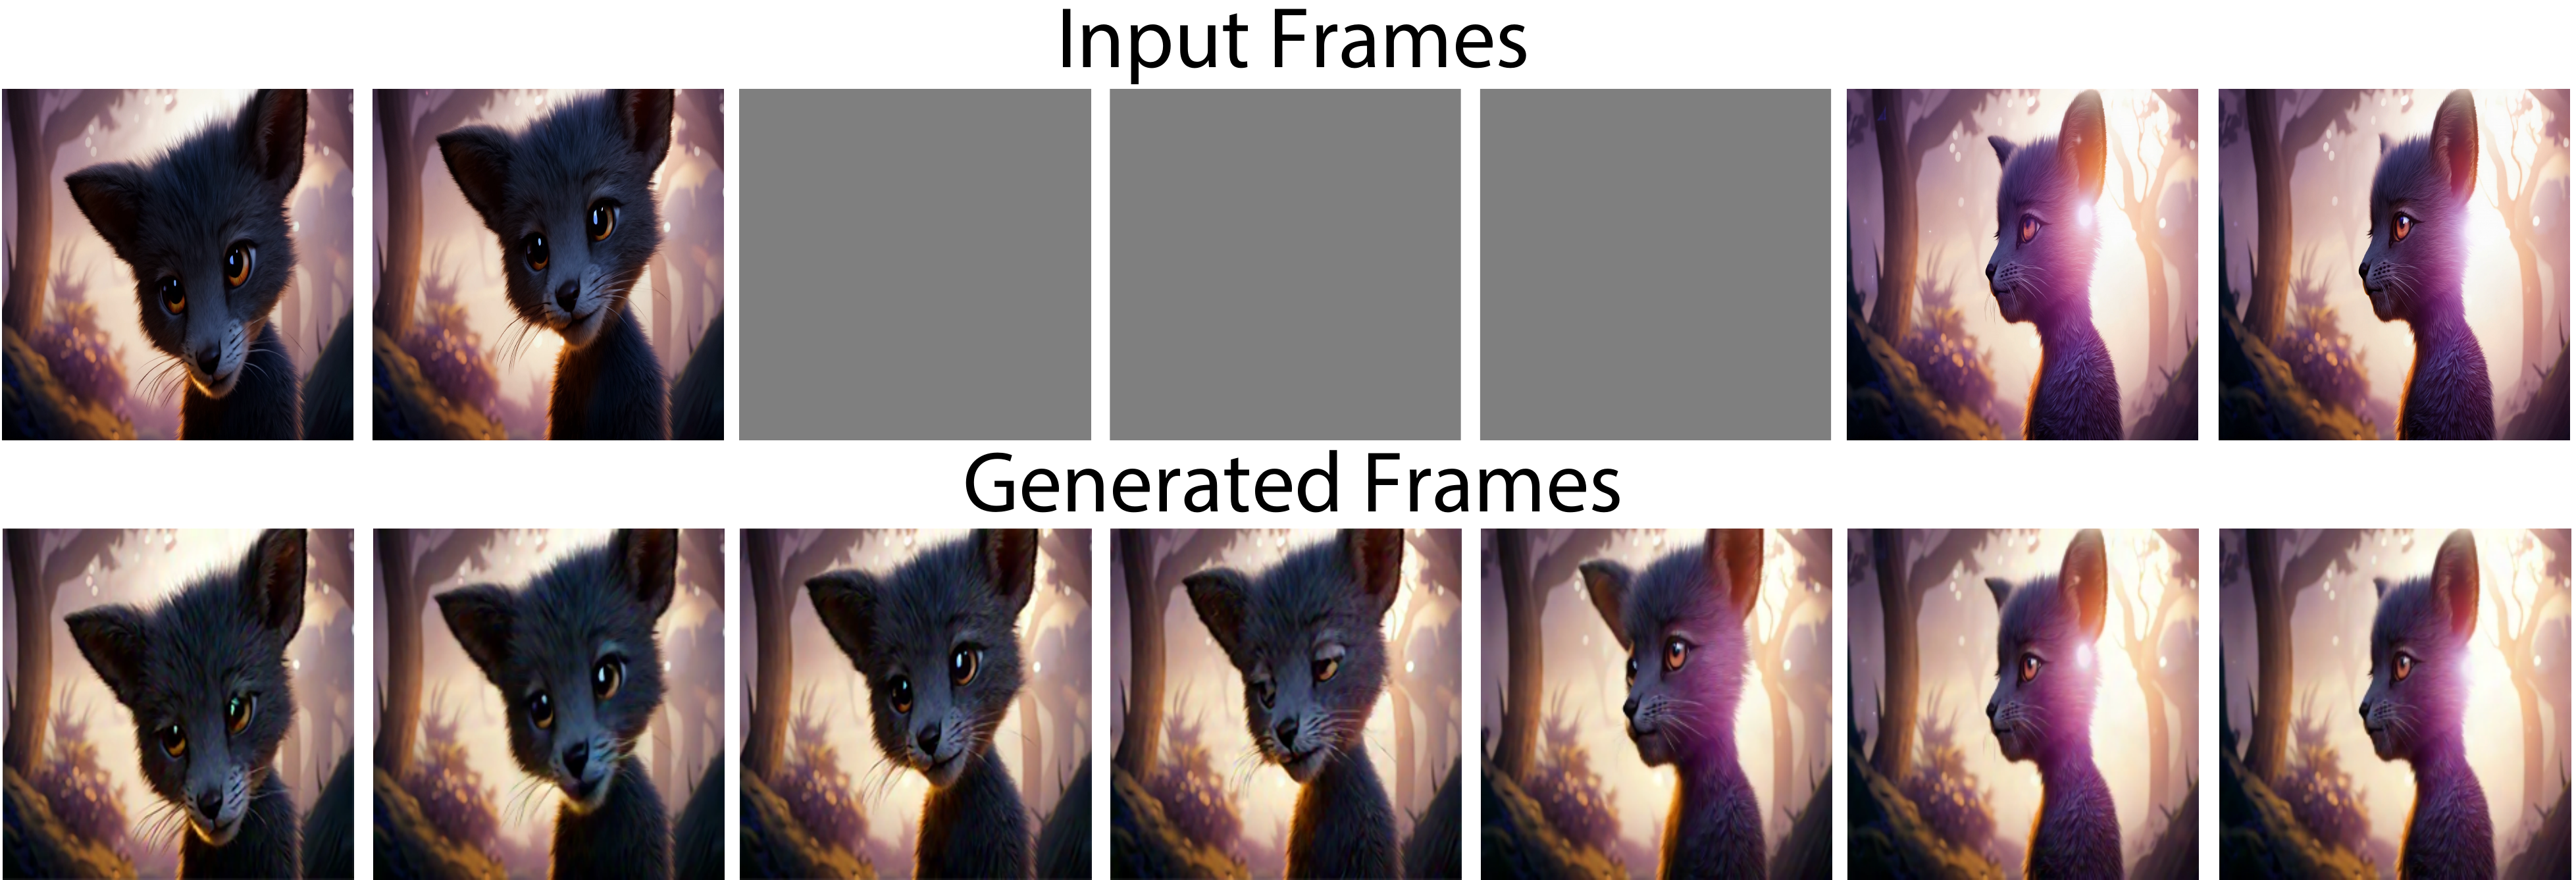}
  \caption{ 
  \mt{Temporal inpainting results: Given an input sequence with missing frames, the generated frames fill in the gaps.}
  }
  \label{fig:temporal}
\end{figure}
\subsection{Video Temporal Inpainting}
\mt{Given a set of video frames with missing frames in between, our model generates the intermediate frames using automatically extracted sparse motion guidance as shown in Fig.~\ref{fig:temporal}}.
